# Supplementary material for: Scaling-up Diverse Orthogonal Convolutional Networks with a Paraunitary Framework
Source: arXiv:2106.09121 source file (2021-06-16)
Supplement: Supplementary file 2 [file supp_packages.tex]

\usepackage{times}
\usepackage[colorlinks=true,linkcolor=blue,citecolor=green,urlcolor=black]{hyperref}
\usepackage[T1]{fontenc}    % use 8-bit T1 fonts
\usepackage{url}            % simple URL typesetting
\usepackage{booktabs}       % professional-quality tables
\usepackage{nicefrac}       % compact symbols for 1/2, etc.
\usepackage{microtype}      % microtypography
\usepackage{xcolor}         % colors

\usepackage{floatrow}
\floatsetup[table]{capposition=top}

\usepackage{caption}
\usepackage{subcaption}

\usepackage{graphicx,float,pgfplots,wrapfig,sidecap,lipsum}
\usepackage{tabularx}
\usepackage{tabulary}
\usepackage{paralist}

\usepackage{array}
\usepackage{makecell}
\usepackage{nomencl}

\usepackage{enumerate}
\usepackage{enumitem}

\usepackage{color}
\usepackage{xcolor}

\usepackage{tablefootnote}
\usepackage{multirow}
\usepackage{diagbox}

\usepackage{xspace}
\usepackage{pifont}
\usepackage{dsfont}
\usepackage{bm}
\usepackage{bbm}
\usepackage{amsfonts}
\usepackage{amsthm}
\usepackage{amssymb}
\usepackage{amsmath}
\usepackage{thmtools,thm-restate}
\usepackage{mathrsfs}
\usepackage{mathtools}
\usepackage{cleveref}

\usepackage{stmaryrd}
\usepackage[utf8]{inputenc}
\usepackage[english]{babel}

% pgfplots
\usepackage[utf8]{inputenc}
\usepackage{pgfplots}
\pgfplotsset{compat=newest}
\usepgfplotslibrary{groupplots}
\usepgfplotslibrary{dateplot}

% tikz
\usepackage{tikz}
\usetikzlibrary{fit}
\usetikzlibrary{calc,shapes}
\usetikzlibrary{decorations.pathmorphing} % noisy shapes
\usetikzlibrary{fit}					% fitting shapes to coordinates
\usetikzlibrary{backgrounds}	% drawing the background after the foreground

%\pgfplotsset{compat=1.17}
